# Supplementary material for: Loan maturity aggregation in interbank lending networks obscures mesoscale structure and economic functions
Source: arXiv:1906.08617 source file (2019-06-12)
Supplement: Supplementary file 1 [file evidence.tex]

\section{Evidence-based OG inference}

\begin{figure}[h] 
\centering
\includegraphics{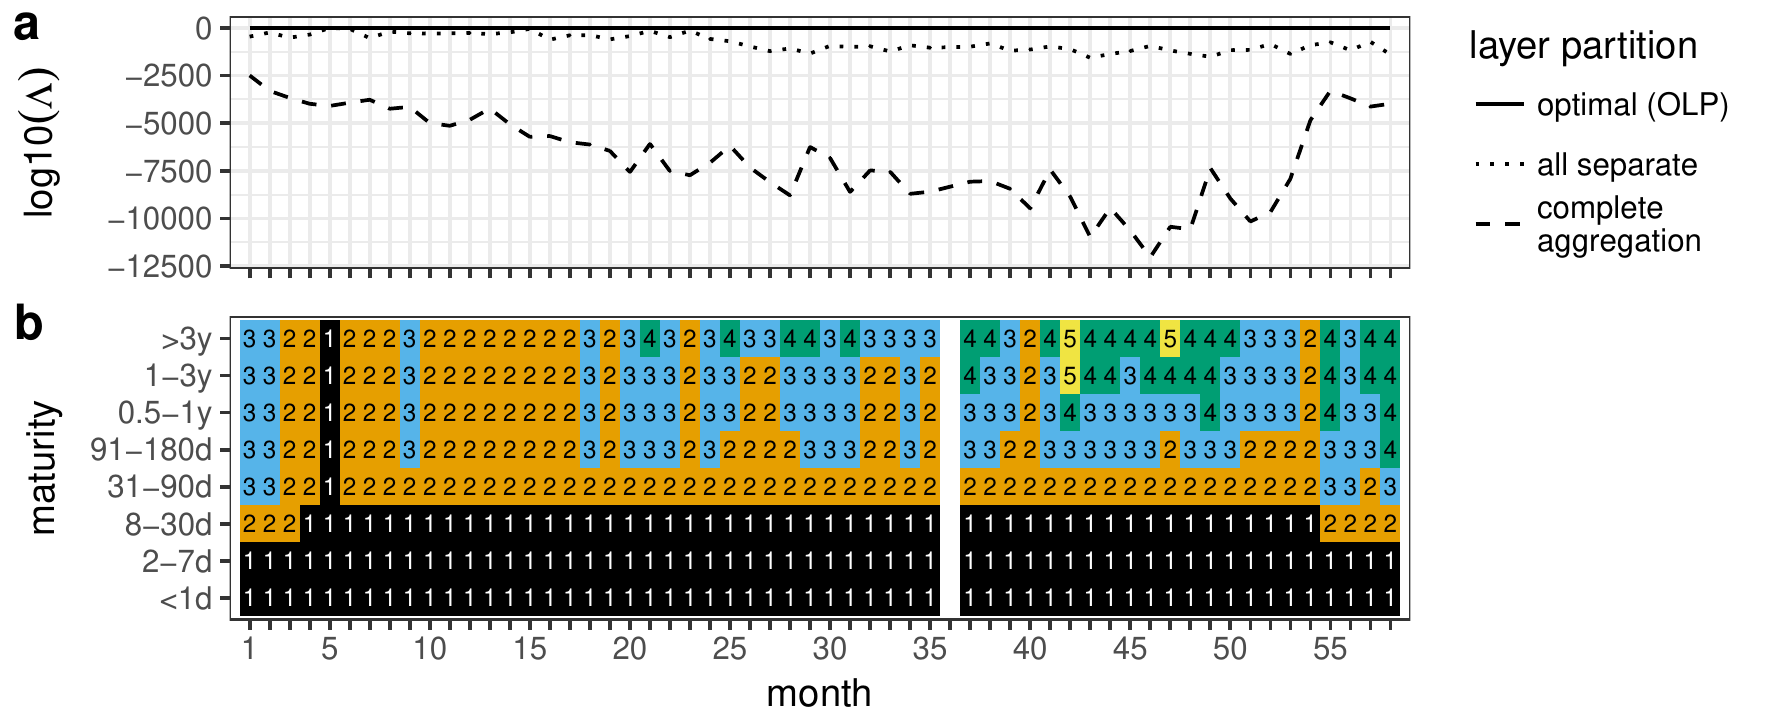}
\caption{Results of the layered SBM with evidence collection. (a) Posterior odds ratios of the OLP compared to two other main cases corresponding resp. to the highest and lowest possible maturity granularity: all layers separate and complete maturity collapse. The latter, though most often used, is always suboptimal to the OLP. (b) The OLP. Maturities with equal color are part of the same (merged) layer in the OLP, also indicated by the number (the Optimal Layer index or OLi).\label{contiguous-evidence}}
\end{figure}

% OLD EVIDENCE NOTES

% Alternatively, ...
% Evidence approach: explain and refer to Appendix C. If evidence approach does not work, perhaps explain why in a subsubsection here and try to figure out why we should be OK with inferring all simultaneously

% OLD NOTES:
% - Optimal granularity based on evidence. Evidence can be only based on RUN9. We take just the minimum DL because (a) is easier to understand because of the similarity to an objective function based approach; (b) The evidence approach rests on the Bethe approximation which requires locally non-tree behavior, a condition not readily satisfied by the network; (c) Because we are searching a non-continuous state space, there are no problems with typicality etc. (We are not optimizing for probability density but for probability mass. But is this actually relevant here?) (d) There are indications of a unimodal pdf over the bank groups. So looking for its maximum is quite sensible.
